# Supplementary material for: A Survey of Secure Computation Using Trusted Execution Environments
Source: arXiv:2302.12150 source file (2023-02-23)
Supplement: Supplementary file 1 [file appendix.tex]

\section{Formal Abstraction} \label{appsec:formal_abstraction}
In this section, we present a formal abstraction of the secure enclave contributed by \cite{pass2017formal}, which is also adopted by the following works for formal security analysis, such as \cite{choudhuri2017fairness, paul2019efficient, wu2022hybrid}. It has been shown that a formal abstraction for enalves has three advantages. Specifically,
\begin{itemize}
    \item {\itshape Formally enables correct usage of trusted hardware.} Extensive works have shown how to build various secure systems with trusted hardware. However, it is still unclear what precise abstraction the trusted hardware provides; the methodology adopted by most existing works goes from heuristic security to semi-formal reasoning.
    \item {\itshape Design user-friendly higher-level programming abstractions.} Clearly, hiding away the cryptographic details will be very attractive for programmers. Formal abstraction may secure the engineering in general and provide possibilities to design user-friendly high-level programming abstractions.
    \item {\itshape Towards formally secure trusted hardware.} Understanding what is a “good” abstraction for trusted hardware can provide useful feedback to the designers and manufacturers of trusted hardware. This may potentially enable us to make sure that the products meet the specification.
\end{itemize}

\begin{figure}[h]
\centering
\begin{mybox}[colback = white, width = 0.85\textwidth]{\text{$\mathcal{G}_{att}[\varSigma, \textsf{reg}]$}}
\gray{\slash\slash \ initialization:} \\
On initialize: $\textsf{(mpk, msk)} \gets \varSigma.\textsf{KeyGen}(1^\lambda)$, $T \gets \emptyset$
\\ \\
\gray{\slash\slash \ public query interface:} \\
On receive $\textsf{getpk}()$ from some $\mathcal{P}$: sends \textsf{mpk} to $\mathcal{P}$
\begin{center}
    \begin{mybox}[colback = white, width = \textwidth]{Enclave Operations}
    \gray{\slash\slash \ local interface -- install an enclave:} \\
    On receive $\textsf{install}(idx, \textsf{prog})$ from some $\mathcal{P} \in \textsf{reg}$:
    \begin{itemize}{}
        \item if $\mathcal{P}$ is honest, assert $idx = sid$
        \item generate a nonce $eid \in \{0, 1\}^\lambda$, store $T[eid, \mathcal{P}] \gets (idx, \textsf{prog}, 0)$
        \item sends $eid$ to $\mathcal{P}$
    \end{itemize}
    ~ \\
    \gray{\slash\slash \ local interface -- resume an enclave:} \\
    On receive $\textsf{resume}(eid, \textsf{inp})$ from some $\mathcal{P} \in \textsf{reg}$:
    \begin{itemize}
        \item let $(idx,\textsf{prog, mem}) \gets T[eid, \mathcal{P}]$, abort if not found
        \item let $\textsf{(outp,mem)} \gets \textsf{prog(inp,mem)}$, update $T[eid,\mathcal{P}] := (idx,\textsf{prog,mem})$
        \item let $\sigma \gets \varSigma.\textsf{Sig}_{\textsf{msk}}(idx,eid,\textsf{prog,outp})$, and send $(\textsf{outp}, \sigma)$ to $\mathcal{P}$
    \end{itemize}
    \end{mybox}
\end{center}
\end{mybox}
\caption{Formal Abstraction of Hardware Enclave.} \label{fig:formal_abstraction}
\Description{Add Description Here.}
\end{figure}

With these benefits, we now present the formal abstraction (also denoted $\mathcal{G}_{att}$), shown in Fig. \ref{fig:formal_abstraction}. $\mathcal{P}$ is the identifier of party. $\textsf{reg}$ refers to the registry of machines with the trusted hardware. \textsf{prog} is the program, which may be probabilistic. $\textsf{inp}$ and $\textsf{outp}$ are the input and output. $\textsf{mem}$ is the program's memory tape. $eid$ is the identifier of an enclave. $\varSigma$ is a signature scheme.  In initialization, the hardware producer generates a key pair $\textsf{(mpk, msk)}$ of signature scheme $\varSigma$ for achieving attestation and initialize a global list $\textsf{reg}$ for managing the parties that are equipped with secure processors. Only the parties in $\textsf{reg}$ has the ability to produce valid attestations. Besides, $\mathcal{G}_{att}$ also provides a public interface $\textsf{getpk}()$, which allows all users to check the validity of attestations. After initialization, $\mathcal{P}$ can load a program $\textsf{prog}$ into enclave by calling ``install'' algorithm and then any user can submit a $\textsf{input}$ to $\mathcal{P}$ and $\mathcal{P}$ obtains the $\textsf{outp} \gets \textsf{prog(input)}$ by invoking ``resume''. It is worth mentioning that the attestation mechanism provides guarantee of correct installation and correct execution of $\textsf{prog}$.

\begin{comment}

\section{Some template}

Appendix goes here ...

%%% -------------- %%%

\begin{figure}[h]
\centering
\begin{mybox}[colback = white, width = 0.9\textwidth]{Title}
Outer box.
    \begin{center}
    \begin{mybox}[colback = white, width = \textwidth]{Title}
    Inner box.
    \end{mybox}
    \end{center}
\end{mybox}
\caption{Box Figure}
\Description{Add Description Here.}
\end{figure}

%%% ------------------ %%%

\begin{figure}[h]
\centering
\begin{tabular}{lr}
\centering
\begin{mybox}[colback = white, width = 0.45\textwidth]{Title}
First box.
\end{mybox}
&
\begin{mybox}[colback = white, width = 0.45\textwidth]{Title}
This is my second box.
\end{mybox}
\\
\multicolumn{2}{l}{
    \begin{mybox}[colback = white, width = \textwidth]{Title}
        Large Box
    \end{mybox}
}
\end{tabular}
\caption{Box Figure}
\Description{Add Description Here.}
\end{figure}

\fullcircle{black}{white}
\halfcircle{black}{white}{90}
\fullcircle{black}{black}

\colorbox{yellow}{Data oblivious}; 

\begin{figure}[h]
  \centering
  \includegraphics[width=0.9\linewidth]{./figs/cmptemplate.png}
  \caption{ Basic Town Crier architecture. Trusted components are depicted in green.}
  \Description{..}
\end{figure}

\end{comment}
